# Supplementary material for: A frequency-independent solver for systems of first order linear ordinary differential equations
Source: arXiv:2309.13848 source file (2023-09-25)
Supplement: Supplementary file 1 [file appendix.tex]

\begin{section}{An adaptive spectral solver for ordinary differential equations}
\label{section:appendix}

In this appendix, we detail a standard  adaptive  spectral method for solving ordinary
differential equations.
It is used by the local Levin method, and to calculate reference
solutions in our numerical experiments. We describe its operation in the 
case of the initial value problem
\begin{equation}
\left\{
\begin{aligned}
\bm{y}'(t) &= F(t,\bm{y}(t)), \ \ \ a < t < b,\\
\bm{y}(a) &= \bm{v}
\end{aligned}
\right.
\label{algorithm:system}
\end{equation}
where $F:\mathbb{R}^{n+1} \to \mathbb{C}^n$ is smooth and $\bm{v} \in \mathbb{C}^n$.
However, the solver can be easily modified to produce a solution with a specified value
at any point $\eta$ in $[a,b]$.

The solver takes as input a positive integer $k$, a tolerance parameter $\epsilon$, an interval $(a,b)$, 
the vector $\bm{v}$ and a 
 subroutine for evaluating the function $F$.  It outputs $n$ piecewise $(k-1)^{st}$ order Chebyshev expansions,
one for each of the components $y_i(t)$ of the solution $\bm{y}$ of (\ref{algorithm:system}).

The solver maintains two lists of subintervals of $(a,b)$: one consisting of what we term ``accepted subintervals''
and the other of subintervals which have yet to be processed.  A subinterval is accepted if the solution
is deemed to be adequately represented by a $(k-1)^{st}$ order Chebyhev expansion on that subinterval.
Initially, the list of accepted subintervals is empty and the list of 
subintervals to process contains the single interval $(a,b)$.
It then operates as follows until the list of subintervals to process is empty:
\begin{enumerate}

\item
Find, in the list of subinterval to process, the interval $(c,d)$ such that
$c$ is as small as possible and remove this subinterval from the list.

\item
Solve the initial value problem
\begin{equation}
\left\{
\begin{aligned}
\bm{u}'(t) &= F(t,\bm{u}(t)), \ \ \ c< t < d,\\
\bm{u}(c) &= \bm{w}
\end{aligned}
\right.
\label{algorithm:ivp2}
\end{equation}
If $(c,d) = (a,b)$, then we take $\bm{w}=\bm{v}$.  Otherwise,
the value of the solution at the point $c$ has already been approximated, and we use that estimate
for $\bm{w}$ in (\ref{algorithm:ivp2}).

If the problem is linear, a straightforward Chebyshev integral equation method 
is used to solve (\ref{algorithm:ivp2}).  Otherwise, 
the trapezoidal method is first used to produce an initial
approximation $\bm{y_0}$ of the solution and then Newton's method is applied to refine it.
The linearized problems are solved using a Chebyshev integral equation method.

In any event, the result is a set of $(k-1)^{st}$ order Chebyshev expansions 
\begin{equation}
u_i(t)  \approx \sum_{j=0}^{k-1} \lambda_{ij}\ T_j\left(\frac{2}{d-c} t + \frac{c+d}{c-d}\right),\ \ \ i=1,\ldots,n,
\label{algorithm:exps}
\end{equation}
approximating  the components $u_1,\ldots,u_n$ of the solution of (\ref{algorithm:ivp2}).

\item
Compute the quantities
\begin{equation}
\frac{\sqrt{\sum_{j=\lfloor k/2 \rfloor+1}^{k-1} \left|\lambda_{ij}\right|^2}}{\sqrt{\sum_{j=0}^{k-1} \left|\lambda_{ij}\right|^2}}, \ \ \ i=1,\ldots,n,
\end{equation}
where the $\lambda_{ij}$ are the coefficients in the expansions (\ref{algorithm:exps}).
If any of the resulting values is  larger than $\epsilon$,
then we split the subinterval into two halves $\left(c,\frac{c+d}{2}\right)$ and 
$\left(\frac{c+d}{2},d\right)$ and place them on the list of subintervals to process.  Otherwise, we place the subinterval
$(c,d)$ on the list of accepted subintervals.

\end{enumerate} 

At the conclusion of this procedure,  we have $(k-1)^{st}$ order piecewise Chebyshev expansions
for each component of the solution, with the list of accepted subintervals determining the
partition for each expansion.

\end{section}
